# Supplementary material for: Demultiplexing through a multimode fiber using chip-scale diffractive neural networks
Source: arXiv:2512.04767 source file (2025-12-04)
Supplement: Supplementary file 1 [file DNN_DEMUX_supplement_20251204.pdf]

# Supplementary Material

# Demultiplexing through a multimode fiber using chip-scale diffractive neural networks

**Qian Zhang[1,+,*], Haoyi Yu[2,+], Jie Zhang[1], Yuedi Zhang[1], Chao Meng[2], Jiali Sun[1], Yu Miao[1], Qiming Zhang[2], Min Gu[2,*], and Juergen W Czarske[1,*]**

[1]Laboratory of Measurement and Sensor System Technique, TU Dresden, Helmholtzstrasse 18, 01069, Dresden, Sachsen, Germany
[2]School of Artificial Intelligence Science and Technology, University of Shanghai for Science and Technology, Shanghai 200093, China
[*]juergen.czarske@tu-dresden.de, qian.zhang@tu-dresden.de, gumin@usst.edu.cn
[+]these authors contributed equally to this work

## Implementation of optical diffractive neural network

Optical diffractive neural network (DNN), first proposed by Lin et al. in 2018, is a physical mechanism used to perform deep learning algorithms for object classification[1]. In contrast to traditional deep neural networks, DNN is an all-optical network model. It consists of multiple diffraction layers, each of which is equivalent to a hidden layer in a conventional neural network, and each unit on the diffraction layer is a neuron. The complex optical field containing information is the input of the DNNs, and the output is the light field modulated by the diffraction layers. According to Huygens' principle, when a beam of coherent light irradiates the diffraction layer of the DNN, each point on the layer will become a secondary wave source. The amplitude and phase of the point wave source depend on the superposition of the incident wave and are modulated by the transmission coefficient at that point. In this way, all neurons on the diffraction layer are connected to each neuron on the subsequent layer. Such a network structure is similar to a fully connected neural network[2] as shown in Figure S1. In forward propagation, as indicated by the red arrow in the figure, the input field is sequentially modulated by all diffractive layers. Backward propagation indicated by the green arrow, is then employed to iteratively update the parameters of each layer by minimizing the error between the predicted and target output fields.

The implementation of DNN consists of two parts: the simulation of optical light propagation and the construction of a trainable model. In this work, the angular spectrum method (ASM) is used to simulate the propagation of light waves. The principle of ASM is based on the theory of Fourier optics, where the light field is processed by converting it from the spatial domain to the frequency domain. The basic idea of the method is to represent an arbitrary complex light field as a superposition of a series of plane waves of the same frequency in different directions[3]. The method involves using the Fast Fourier Transform (FFT) to decompose the light field into plane waves, propagating each component separately, and then applying the Inverse Fast Fourier Transform (IFFT) to reconstruct the propagated light field.

Assuming that the distribution of the light field in the $z=0$ plane is $U(x,y,0)$, the initial light field is Fourier transformed to obtain the angular spectral distribution of the light field in the frequency domain $U(f_x,f_y,0)$ in the $z=0$ plane:

$$U(f_x,f_y,0)=\iint_{-\infty}^{+\infty} U(x,y,0)e^{-j2\pi(f_x x+f_y y)}\,dx\,dy, \tag{1}$$

where $f_x$ and $f_y$ denote the spatial frequencies. When the optical field propagates to $z$ along the propagation direction, its angular spectral distribution $U(f_x,f_y,z)$ can be obtained by multiplying the FT of the initial field by the phase coefficient $e^{jk_z z}$:

$$U(f_x,f_y,z)=U(f_x,f_y,0)\cdot e^{jk_z z}. \tag{2}$$

Here, $k_z$ is a function of spatial frequency:

$$k_z=\sqrt{k^2-(2\pi f_x)^2-(2\pi f_y)^2}, \tag{3}$$

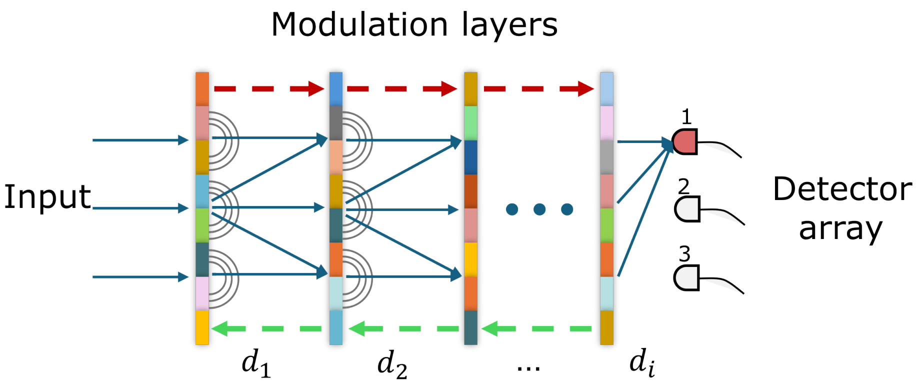


**Figure S1.** Model of optical diffractive deep neural network. $d_i$ indicates the distance between adjacent layers and the distance between the last layer and the detector.

where $k = 2\pi/\lambda$ is the wave number and $\lambda$ is the wavelength of the light wave. When $k^2 \geq (2\pi f_x)^2 + (2\pi f_y)^2$, $k_z$ is a real number, which means the light field is in propagating mode and propagates normally in space; when $k^2 < (2\pi f_x)^2 + (2\pi f_y)^2$, $k_z$ is an imaginary number, which means that the light field is in evanescent mode, and it will be fading fast during propagation.

The IFFT of the angular spectrum at $z$ converts the angular distribution in the frequency domain back to the spatial domain to obtain the light field distribution $U(x,y,z)$ at propagation distance $z$:

$$U(x,y,z) = \iint_{-\infty}^{+\infty} U(f_x, f_y, z) e^{j2\pi(f_x x + f_y y)} \, df_x \, df_y. \tag{4}$$

In the construction of one DNN, to guarantee the optical information transfer between adjacent layers, a fully connected topology is used during the design of the DNN[1]. Each neuron, the micro-structure unit, on the diffraction layer of DNN is connected to all neurons on the next diffraction layer. In order to enable this full connectivity by diffraction, the angle of diffraction at the neuron needs to be specifically designed. According to the diffraction grating equation:

$$2d \cdot \sin(\varphi_{\max}) = m \cdot \lambda, \tag{5}$$

where $d$ is the grating spacing (the size of one unit pixel), $m$ is the diffraction order, $\varphi_{\max}$ is the maximum diffraction angle, which can be calculated when $m = 1$:

$$\varphi_{\max} = \sin^{-1}\left(\frac{\lambda}{2d}\right). \tag{6}$$

From the Equation 6, it can be seen that the maximum diffraction angle can be determined by the wavelength and the pixel spacing. In general, a longer wavelength and a smaller neuron size are welcome to provide more sufficient full connections in DNN. However, it should be noted that the maximum is 90° when the grating spacing $d$ is $\frac{\lambda}{2}$. However, if $d < \frac{\lambda}{2}$ it enters the subwavelength regime, where diffraction is suppressed.

For the design of the structure of DNNs, the relationship between the wavelength, neuron size, and the layer distance should be clarified. If the layer distance between two adjacent layers is $d_l$, the radius of the diffraction spot of each neuron is then:

$$R_d = d_l \cdot \tan(\varphi_{\max}). \tag{7}$$

Assuming that the diffraction layer is square, the DNN can achieve full connectivity if $R_d \geq \sqrt{N_{\text{layer}}} \cdot d_p$. Therefore, the $d_l$ should satisfy:

$$\begin{cases} \varphi_{\max} = \sin^{-1}\left(\dfrac{\lambda}{2d_p}\right), \\ d_l \geq \sqrt{N_{\text{layer}}} \cdot d_p \sqrt{\left(\dfrac{2d_p}{\lambda}\right)^2 - 1}. \end{cases} \tag{8}$$

The above formula shows that the connectivity of DNNs is related to the layer distance, wavelength, neuron size, and the number of neurons. In the real experiments, the wavelength and the smallest neuron size are often hard to change. Therefore, it is more convenient to adjust the layer distance and the layer size to optimize the connectivity. In this work, the neuron size is 1 µm, which is determined by the fabrication setup. As the fiber used has a diameter of 25 µm, the field size in simulation is set as 25 × 25 pixels. Taking into account the spreading of the optical field during propagation, the layer size is chosen to be 120 µm. The layer distance is 40 µm.

## Characterization of multimode fiber (MMF)

The characterization of MMF used in the experimental setup is crucial to make the 3D-printed DNN working correctly. One approach is to decompose experimentally measured modal field distributions. Based on the decomposed modal weights, a comparison between the reconstruction and measured images can be conducted. The higher the correlation coefficient of the reconstruction, the more precisely the mode profile with the corresponding mode weights can be determined. In this work, we build a deep neural network and generate a training dataset consisting of pure synthetic data. We first generate a large number of random modal weights. The amplitudes satisfy energy normalization, and the relative phases are uniformly sampled from $[0, 2\pi)$, with the fundamental mode used as the reference. These random weights are then combined with the theoretical LP mode fields through linear coherent superposition, and the intensity is obtained by taking the squared magnitude of the field. The entire dataset is synthetic, and the network is trained without using any experimental data.

Although the network is trained only in the simulation domain, its goal is to demultiplex experimentally recorded speckle patterns. Since experimental images differ from simulated ones in terms of pixel values, noise levels, and background structure, they must be preprocessed before use for prediction. This includes cropping to extract the effective core region and normalizing the intensity to match the dynamic range of the simulated data. These steps help align the statistical features of the experimental images with those in the training domain.

With this procedure, the trained Mode Transformer Network (MTNet)[4] can take preprocessed experimental intensity images and predict the corresponding modal amplitudes and relative phases. By learning the mapping from intensity patterns to modal weights using large-scale synthetic data, the network can perform reliable mode decomposition on unlabeled experimental images and recover the energy distribution inside the fiber.

## Training of deep neural network model for reference-free mode decomposition

In this study, we used MTNet[4] as the deep-learning model to predict the modal amplitudes and relative phases from simulated intensity images. The model is based on a small Vision Transformer[5], which includes a 128-dimensional embedding, three Transformer blocks, four attention heads, and a 256-dimensional MLP layer. The input image size is $50 \times 50$, and the patch size is set to 50 so that the entire image is treated as one token. The training dataset contains 300,000 simulated intensity images. The network is trained from scratch on a single NVIDIA RTX A6000 GPU and reaches convergence after about 315 minutes. After training, we evaluate the model on 1,000 independent simulated test samples. The results show that the predicted modal weights have more than 99% similarity with the ground truth. This indicates that MTNet can learn the nonlinear mapping between intensity patterns and modal parameters and provides a reliable basis for reference-free modal decomposition on experimental data. It should be noted, such a data-driven model can perform well in decomposition on less than tens of modes. For more modes, a physics-informed neural network can be used[6].

## Improved numerical simulation of free-space propagation

To mitigate unphysical wrap-around artefacts during free-space propagation, we follow the rationale of the band-limited angular spectrum method by Matsushima and Shimobaba[7] and explicitly enlarge the computational aperture. When the propagation distance is short and the diffracted field remains well confined within the numerical window, such wrap-around is negligible. However, for longer propagation distances or strongly diffracting fields, the optical field can expand beyond the original aperture so that energy leaving one side of the window would re-enter from the opposite side due to the implicit periodic boundary conditions of the Fourier solver. To prevent this, we embed each optical field within an expanded computational window before every numerical propagation step. This introduces a guard band of zero amplitude surrounding the physical pupil and allows the free-space transfer function to be applied over a larger area, so that diffracted energy near the boundaries decays within the padding instead of folding back into the active region. After each propagation or diffractive modulation, the central region corresponding to the actual device aperture is cropped and forwarded to the next layer, see Figure S2.

This padding strategy leaves the learnable phase masks themselves unchanged, but it effectively suppresses edge aliasing and ensures that the reconstructed intensity distributions correspond to a physically realistic, non-periodic propagation model.

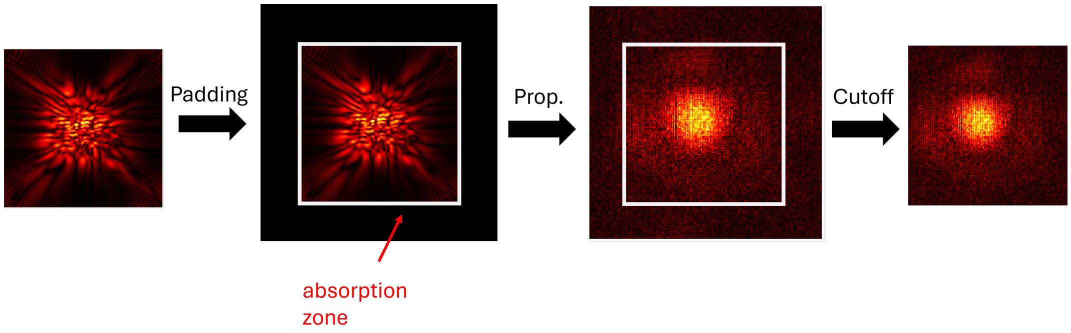


**Figure S2.** Padding-based suppression of wrap-around artefacts during free-space propagation.

## Influences of phase distribution on the performance of diffractive neural network

The light field emerging from a multimode fiber is a complex field with amplitude and phase distribution. During the training of DNN, only the eigenmodes are utilized. The output of the DNN represents the proportion of energy of the different modes, i.e., the squares of modal amplitude weights. Here, we discuss the effect of phase distribution on the results of DNN-based DEMUX. Two different scenarios are considered: the first one is where the mode amplitude weights are fixed, but the relative phase is randomized. As shown in Figure S3, the superimposed light fields differ in intensity distribution due to the relative phase. However, the DNN can demodulate the optical light field well with accurate amplitude weights of each mode. This result implies that the DNN can overcome the effect of phase on the optical field distribution to accurately demodulate the fiber output when faced with a random superimposed optical field. However, this does not mean that the phase distribution is negligible. Another test with non-phase distribution information was conducted. The phase distribution of the superimposed light field is set to 0. In this case, when the light field passes through the DNN, almost all the energy is concentrated in the first detection region, see Figure S4. The DNN outputs similar results despite the fact that the intensity distribution of the light field is quite different due to different combinations of mode weights. The main reason for this is that the first eigenmode $LP_{01}$ has a plane phase distribution. Therefore, when the phase distribution of the light field is forced to zero, the DNN erroneously converges the light field to the region of the first mode.

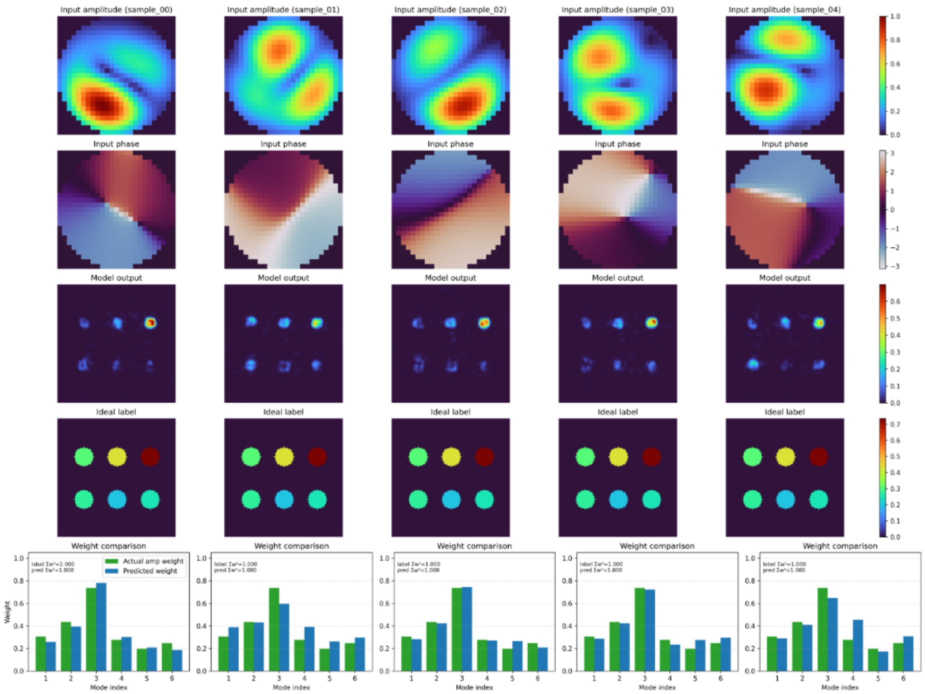


**Figure S3.** Demultiplexing of mode superpositions with constant amplitude weights and varied relative phases.

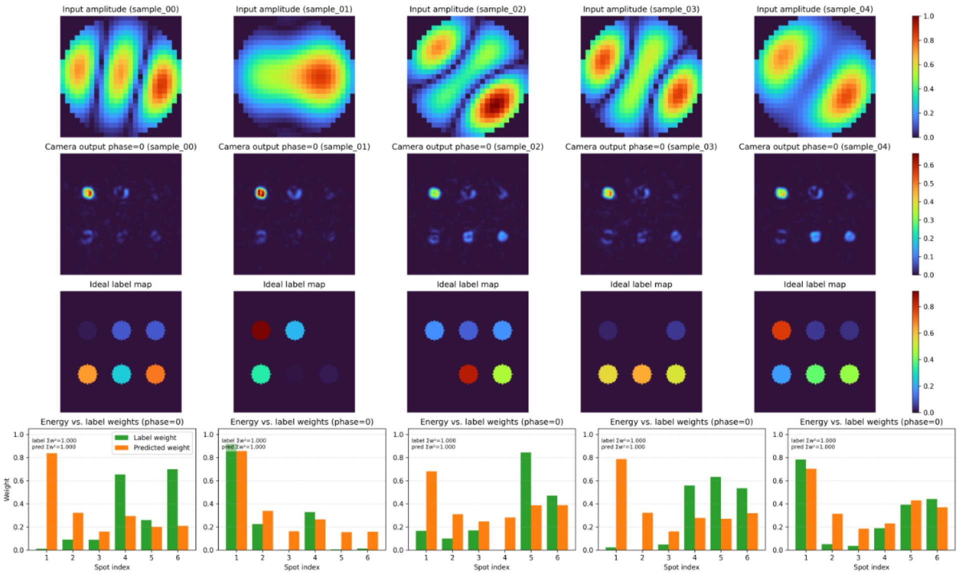


**Figure S4.** Demultiplexing of mode superpositions with random modal weights. The phase distribution is set as 0.

## Experimental setup

The schematic of the setup is shown in Supplementary Figure S5. The laser output is delivered through a polarization-maintaining single-mode fiber (PM-SMF) to a fiber port (PAF2S-11C), a highly compact coupling stage that injects the free-space laser beam efficiently into the multimode fiber (step-index MMF, M68L02). The distal end of the MMF is left as a bare fiber and mounted on a precision 3-axis translation stage (MBT616D/M), which provides fine control of both the lateral launch position into the ODNN-AMD and the axial spacing between the MMF facet and the first diffractive layer. To further facilitate alignment, an imaging path is incorporated into the setup for real-time monitoring. In this monitoring path, the LED illuminates the ODNN-AMD and the MMF fiber facet, and their interface region is imaged by MO2 (M PLAN APO NIR 20X) and L2 onto CAM2 (Basler ace 2 R Basic), providing continuous visualization of the alignment conditions. To image the results of the ODNN-based mode demultiplexer, a 20× near-infrared microscope objective (M PLAN APO NIR 20X) and an achromatic lens (AC254-100-C-ML) are used to form the imaging path that collects and magnifies the output field. The modulated optical field produced by the ODNN-AMD is then captured by an InGaAs camera (Alvium G1-030 VSWIR), which provides high sensitivity at the operating wavelength of our system. A tunable CW laser source (CBDX1-1-GC-FA) serves as the illumination input for all experiments. Together, these components form a compact and mechanically stable optical platform that enables excitation of MMF modes, controlled injection into the diffractive neural network, and high-fidelity detection of the demultiplexed modal intensities under realistic experimental conditions.

## References


1. Lin, X. *et al.* All-optical machine learning using diffractive deep neural networks. *Science* **361**, 1004–1008 (2018).
2. Sheng, H. Review of integrated diffractive deep neural networks. *Highlights Sci. Eng. Technol.* **24**, 264–278, DOI: 10.54097/hset.v24i.3957 (2022).
3. Goodman, J. W. *Introduction to Fourier optics* (Roberts and Company publishers, 2005).
4. Zhang, Q., Rothe, S., Koukourakis, N. & Czarske, J. Learning the matrix of few-mode fibers for high-fidelity spatial mode transmission. *APL Photonics* **7** (2022).
5. Dosovitskiy, A. An image is worth 16x16 words: Transformers for image recognition at scale. *arXiv preprint arXiv:2010.11929* (2020).
6. Zhang, Q., Sui, Y., Rothe, S. & Czarske, J. Physics-informed mode decomposition neural network for structured light in multimode fibers. In *2023 IEEE Photonics Conference (IPC)*, 1–2 (IEEE, 2023).
7. Matsushima, K. & Shimobaba, T. Band-limited angular spectrum method for numerical simulation of free-space propagation in far and near fields. *Opt. express* **17**, 19662–19673 (2009).

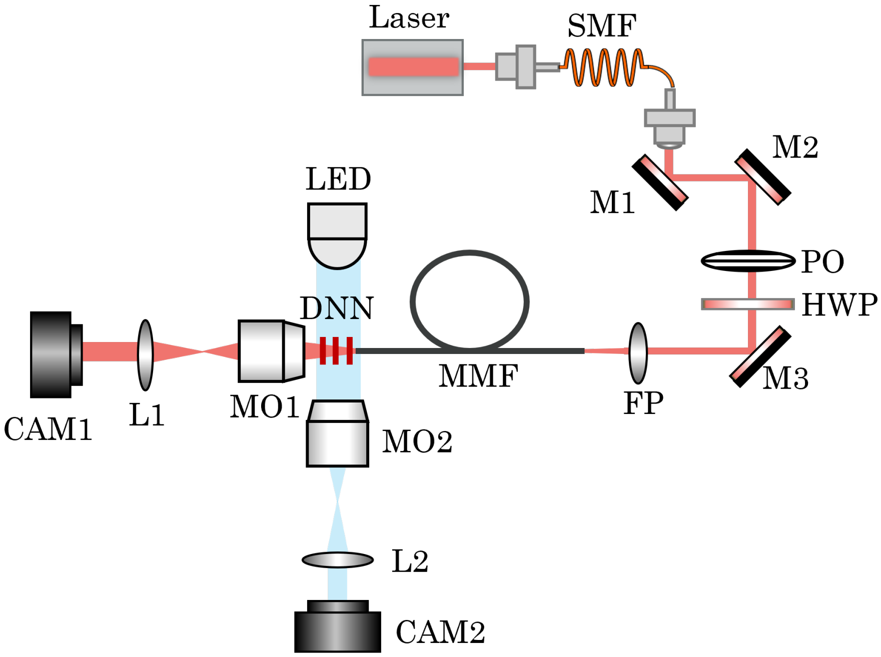


**Figure S5.** Schematic of the experimental setup for DNN-based mode demultiplexing. Abbreviations: CAM, camera; L, lens; MMF, multi-mode fiber; MO, microscope objective; FP: fiber port; HWP: Half wave plate; PO: polarizer; and SMF, single-mode fiber. In this work, a MMF supporting 6 modes @1568 nm were tested.
